# Supplementary material for: MODS: Moderating a Mixture of Document Speakers to Summarize Debatable Queries in Document Collections
Source: arXiv:2502.00322 source file (2025-02-01)
Supplement: Supplementary file 1 [file efficiency_main.tex]

\begin{table}[]
\small
\centering
\begin{tabular}{@{}l|cc|cc@{}}
\toprule
\multicolumn{1}{c|}{\textbf{Model}} & \textbf{GPT-4 Cost} & \textbf{Time in Seconds} & \textbf{DC All} & \textbf{DC Topic} \\ \midrule
\modelTopic & \textbf{0.55} & \textbf{139} & \textbf{0.938} & \textbf{0.587} \\
\modelTopic - Moderator & - & - & - & - \\
Hierarchical-Topic & - & - & - & - \\
Incremental-Topic & 0.71 & 187 & 0.644 & 0.415 \\ \bottomrule
\end{tabular}
\end{table}
