# Supplementary material for: MODS: Moderating a Mixture of Document Speakers to Summarize Debatable Queries in Document Collections
Source: arXiv:2502.00322 source file (2025-02-01)
Supplement: Supplementary file 2 [file prompts.tex]

\hypersetup{
    colorlinks=true, % Enable colored links
    linkcolor=white, % Default color for internal links (sections, etc.)
    citecolor=white, % Default color for citations
    urlcolor=white % Default color for external URLs
}

\begin{prompt}[title={Prompt \thetcbcounter: Agenda Planner Prompt (\cref{subsection:agenda})}, label=prompt:agenda]
The following are documents related to the query: $q$\\
\texttt{$\mathcal{B}$} \\
Based on the documents, produce $m$ fine-grained discussion points discussed in these documents. The discussions point should be short, around 5 words. They should be much more specific than the query, capturing high-level themes or arguments. Avoid overly broad terms like 'Impacts' or 'Benefits'; instead, provide focused terms that are still high-level themes. Your final output must be a JSON dictionary with keys for ``discussion point 1\'', ..., ``discussion point $m+1$''"
\end{prompt}

\begin{prompt}[title={Prompt \thetcbcounter: Speaker Selection Prompt (\cref{subsection:moderator})}, label=prompt:moderator]
The following are documents related to the discussion point: $t_j$\\
\texttt{$\mathcal{B}_j$} \\
Based on the documents, classify which documents may contain useful information and diverse perspectives related to ``$t_j$''. Your final output must be a JSON dictionary with a key for ``relevant documents'', containing a list of integers corresponding to the documents relevant to the point.
For every document, generate a very short question that you think the document is an expert in and captures the perspective of the document related to $t_j$.
Each question should be in the form ``Document N Question:'' as a key in the JSON file, where N is the number of one of the documents.
\end{prompt}

\begin{prompt}[title={Prompt \thetcbcounter: Speaker Discussion Prompt (\cref{subsection:speaker})}, label=prompt:speaker]
The following is a document related to the query: $q$\\
$\mathcal{C}$ \\
Using the document, generate two lists of factual sentences, a ``yes'' list and ``no'' list, related to the query. The ``yes'' list should only contain facts for why the answer to the query under the discussion point is yes, and the ``no'' list should only contain facts for why the answer to the query under the discussion point is no. The lists for yes facts or no facts should be empty if no fact for that answer exists. "
Only produce facts that are directly related to discussion point of ``$t_j$'' and the subquestion of ``$q_{i, j}$''. Your final output must be a JSON dictionary with keys ``discussion point'' for the discussion point, ``yes facts'' for the list of yes facts, and ``no facts'' for the list of no facts"
\end{prompt}

\begin{prompt}[title={Prompt \thetcbcounter: Full Outline Summarization Prompt (\cref{subsection:summary})}, label=prompt:full]
The following is an outline for the query $q$, broken down into $m$ fine-grained discussion points. Under the discussion point, there is a list of documents and a subquestion explaining the document's expertise on the discussion point. Under each document and question, there will be a bullet point list of facts preceded by either ``Yes Fact:'' and ``No Fact:'', denoting whether the fact gives evidence for why the answer to the query is yes or no:\\
$\mathcal{O}$ \\
Synthesize the Yes Facts and No Facts from the outline and produce a brief summary that answers the query under the same $m$ discussion points. The summary should be one brief, three-sentence paragraph per point. Each sentence in the paragraph should include a citation, in the form of a number inside square brackets, indicating the source documents from which the information was derived. Use as many documents as possible. Your final output must be a JSON dictionary with keys for ``discussion point 1:'', ``summary 1:'', ..., `discussion point $m+1$:'', ``summary $m+1$:''.
\end{prompt}

\begin{prompt}[title={Prompt \thetcbcounter: Topic-Level Outline Summarization Prompt (\cref{subsection:summary})}, label=prompt:topic]
The following is an outline for the query $q$ and a single discussion point. Under the discussion point, there is a list of documents and a subquestion explaining the document's expertise on the discussion point. Under each document and question, there will be a bullet point list of facts preceded by either ``Yes Fact:'' and ``No Fact:'', denoting whether the fact gives evidence for why the answer to the query is yes or no:\\
$\mathcal{O}_j$ \\
Synthesize the Yes Facts and No Facts from the outline and produce a brief summary that answers the query under the same discussion point. The summary should be one brief, three-sentence paragraph. Each sentence in the paragraph should include a citation, in the form of a number inside square brackets, indicating the source documents from which the information was derived. Use as many documents as possible. Your final output must be a JSON dictionary with keys for ``discussion point'' and ``summary''.
\end{prompt}

\begin{prompt}[title={Prompt \thetcbcounter: Long-Context Summarization Prompt (\cref{subsection:summary})}, label=prompt:lc]
The following are documents for the query: $q$\\
$\mathcal{D}$\\
Synthesize the facts from the document and produce a brief summary that answers the query under $m$ fine-grained discussion points. The summary should have one brief, three-sentence paragraph per point. Each sentence in the paragraph should include a citation, in the form of a number inside square brackets, indicating the source documents from which the information was derived. Use as many documents as possible. The discussions point should be short, around 5 words. They should be much more specific than the query, capturing high-level themes or arguments. Avoid overly broad terms like 'Impacts' or 'Benefits'; instead, provide focused terms that are still high-level themes. Your final output must be a JSON dictionary with keys for ``discussion point 1:'', ``summary 1:'', ..., `discussion point $m+1$:'', ``summary $m+1$:''.
\end{prompt}

\clearpage

\begin{prompt}[title={Prompt \thetcbcounter: RAG Summarization Prompt (\cref{subsection:summary})}, label=prompt:rag]
The following are documents for the query: $q$\\
$\mathcal{C}$\\
Synthesize the facts from the document and produce a brief summary that answers the query under $m$ fine-grained discussion points. The summary should have one brief, three-sentence paragraph per point. Each sentence in the paragraph should include a citation, in the form of a number inside square brackets, indicating the source documents from which the information was derived. Use as many documents as possible. The discussions point should be short, around 5 words. They should be much more specific than the query, capturing high-level themes or arguments. Avoid overly broad terms like 'Impacts' or 'Benefits'; instead, provide focused terms that are still high-level themes. Your final output must be a JSON dictionary with keys for ``discussion point 1:'', ``summary 1:'', ..., `discussion point $m+1$:'', ``summary $m+1$:''.
\end{prompt}

\begin{prompt}[title={Prompt \thetcbcounter: Hierarchical Summarization Prompt (Intermediate Summary) (\cref{subsection:summary})}, label=prompt:h1]
The following is a document for the query: $q$\\
$\mathcal{D}$\\
\\
Synthesize the facts from the document and produce a summary that answers the query. Your final output must be a JSON dictionary with a key for ``summary''.
\end{prompt}

\begin{prompt}[title={Prompt \thetcbcounter: Hierarchical Summarization Prompt (Merge Summaries) (\cref{subsection:summary})}, label=prompt:h2]
The following are documents for the query: $q$\\
$\mathcal{S}'$\\
Synthesize the facts from the document and produce a brief summary that answers the query under $m$ fine-grained discussion points. The summary should have one brief, three-sentence paragraph per point. Each sentence in the paragraph should include a citation, in the form of a number inside square brackets, indicating the source documents from which the information was derived. Use as many documents as possible. The discussions point should be short, around 5 words. They should be much more specific than the query, capturing high-level themes or arguments. Avoid overly broad terms like 'Impacts' or 'Benefits'; instead, provide focused terms that are still high-level themes. Your final output must be a JSON dictionary with keys for ``discussion point 1:'', ``summary 1:'', ..., `discussion point $m+1$:'', ``summary $m+1$:''.
\end{prompt}

\begin{prompt}[title={Prompt \thetcbcounter: Incremental Summarization Prompt (Merge Summaries) (\cref{subsection:summary})}, label=prompt:i1]
The following is a document related to the query: $q$\\
$\mathcal{D}$\\
The following text contains $m$ current discussion points and summaries:\\
$S_{int}$\\
Synthesize the facts from the document and add to the current summaries under the discussion points. The summary under each point should have a maximum length of one paragraph. If the document has no information that is relevant to the discussion points, that discussion point's summary should remain unchanged. The discussions point should be short, around 5 words. They should be much more specific than the query, capturing high-level themes or arguments. Avoid overly broad terms like 'Impacts' or 'Benefits'; instead, provide focused terms that are still high-level themes. Each new sentence in the paragraph based on the current document should include a citation, in the form of a number inside square brackets, indicating the source document from which the information was derived. The input document has document number $i$, which is the number that should be used for citing information from the input document. Use as many documents as possible. Your final output must be a JSON dictionary with keys for ``discussion point 1:'', ``summary 1:'', ..., `discussion point $m+1$:'', ``summary $m+1$:''.
\end{prompt}

\begin{prompt}[title={Prompt \thetcbcounter: Incremental Summarization Prompt (Self-Refine Summary) (\cref{subsection:summary})}, label=prompt:i2]
The following is a summary for the query: $q$, broken down into $m$ fine-grained discussion points. Under each discussion point is a paragraph related to the query and point:
$\mathcal{S}$ \\
Refine the summary so it is only one brief, three-sentence paragraph. Each sentence in the paragraph should include a citation, in the form of a number inside square brackets, indicating the source documents from which the information was derived. Use as many documents as possible. Your final output must be a JSON dictionary with keys for ``discussion point 1:'', ``summary 1:'', ..., `discussion point $m+1$:'', ``summary $m+1$:''.
\end{prompt}

\begin{prompt}[title={Prompt \thetcbcounter: Incremental Summarization Prompt (Self-Refine Topic Paragraph) (\cref{subsection:summary})}, label=prompt:i3]
The following is a summary for the query $q$ under the discussion point of $t_j$:\\
$\mathcal{S}_j$ \\
Refine the summary so it is only one brief, three-sentence paragraph. Each sentence in the paragraph should include a citation, in the form of a number inside square brackets, indicating the source documents from which the information was derived. Use as many documents as possible. Your final output must be a JSON dictionary with keys for ``discussion point'' and ``summary''. 
\end{prompt}

\clearpage

\begin{prompt}[title={Prompt \thetcbcounter: Cluster Summarization Prompt (\cref{subsection:summary})}, label=prompt:cluster]
The following are documents for the query: $q$\\
$\mathcal{D}$\\
Synthesize the facts from the document and produce a brief summary that answers the query under $m$ fine-grained discussion points. The summary should have one brief, three-sentence paragraph per point. Each sentence in the paragraph should include a citation, in the form of a number inside square brackets, indicating the source documents from which the information was derived. Use as many documents as possible. The discussions point should be short, around 5 words. They should be much more specific than the query, capturing high-level themes or arguments. Avoid overly broad terms like 'Impacts' or 'Benefits'; instead, provide focused terms that are still high-level themes. Your final output must be a JSON dictionary with keys for ``discussion point 1:'', ``summary 1:'', ..., `discussion point $m+1$:'', ``summary $m+1$:''.
\end{prompt}

\begin{prompt}[title={Prompt \thetcbcounter: GPT Entailment Prompt (\cref{subsection:citation_comp})}, label=prompt:cite_acc]
The following are contexts:\\
$\mathcal{C}$ \\
Here is a sentence: $s$\\
Is there a part of this sentence that is supported by the information in the contexts? Answer with just ``Yes'' or ``No''. Your output must be a JSON with the key ``label''
\end{prompt}
